# Supplementary material for: PITA: Preference-Guided Inference-Time Alignment for LLM Post-Training
Source: arXiv:2507.20067 source file (2025-11-13)
Supplement: Supplementary file 1 [file related-work-supp.tex]

\section{Related Work}
\paragraph{Alignment:}
Large language models (LLMs) have been shown to demonstrate emerging capabilities in advanced natural language tasks through the use of the attention mechanism, and the transformer architecture\cite{vaswani2017attention,radford2019language,brown2020language,devlin2018bert,bubeck2023sparks}. In the context of LLMs, the end goal is to fine-tune the responses generated by LLMs for downstream tasks. Reinforcemnt Learning from Human Feedback (RLHF) \cite{christiano2017deep,ziegler2019fine,stiennon2020learning,ouyang2022training} has emerged as a significant technique in aligning LLMs with human values and preferences. Pivotal to the RLHF approach is access to a ground-truth reward model (pre-trained model from preference data or labels from supervised data). An alternative approach to utilize preference information is using Direct Preference Optimization~\cite{rafailov2023direct} to update the model's policy directly using preference data.

\paragraph{LLM Reasoning:}
Recent methodologies further extend the abilities of LLMs to generate intermediate reasoning steps. The standard setup in LLM-based reasoning is to start with an initial policy $\pi$ instantiated by a reference LLM. The output is generated as a sequence of steps by auto-regressively predicting the next step using prompting. The idea is made well-known using the Chain-of-Thought~\cite{wei2022chain} approach to reasoning tasks. Self-Consistency~\cite{wang2022self} choses the most frequent answer among multiple generations. Tree-of-Thought~\cite{yao2023tree} extends the idea of CoT method to generate tree-based reasoning traces encouraging exploration among many possible thoughts. Another idea is to use a value function to guide the otherwise combinatorially large selection of reasoning traces. Two common approaches include Outcome Reward models (ORMs)~\cite{cobbe2021training}, and Process Reward Models (PRMs)~\cite{li2024process}. While ORMs are trained only on the accuracy of the final answer, PRMs are trained on the accuracy of intermediate reasoning steps. A popular approach is to use Best-of-N~\cite{lightman2023let} which combines the utility of a value function (PRM or ORM) by selecting the reasoning trace with the highest value.

% \paragraph{Preference Learning:}
% \bluetext{Come back to working on this paragraph}
% Preference learning has a long history in reinforcement learning, and bandits literature. In addition to the empirical success of training of Large language models to generate outputs aligned with human preferences, the theoretical aspects of preference learning have been extensively studied. The reward-based methods have been proven to be unstable and in general relative preference is easier to obtain in comparison to an absolute reward score.
% Several works characterize the alignment problem as a general preference optimization objective. We discuss preference based methods as is the focus of our work. In ~\cite{azar2024general}, the authors define a general objective for RLHF, of which the RLHF and DPO objectives are a specific example of.
